# Supplementary material for: GEMS: Scene Expansion using Generative Models of Graphs
Source: arXiv:2207.03729 source file (2022-07-08)
Supplement: Supplementary file 1 [file baseline_supp2.pdf]

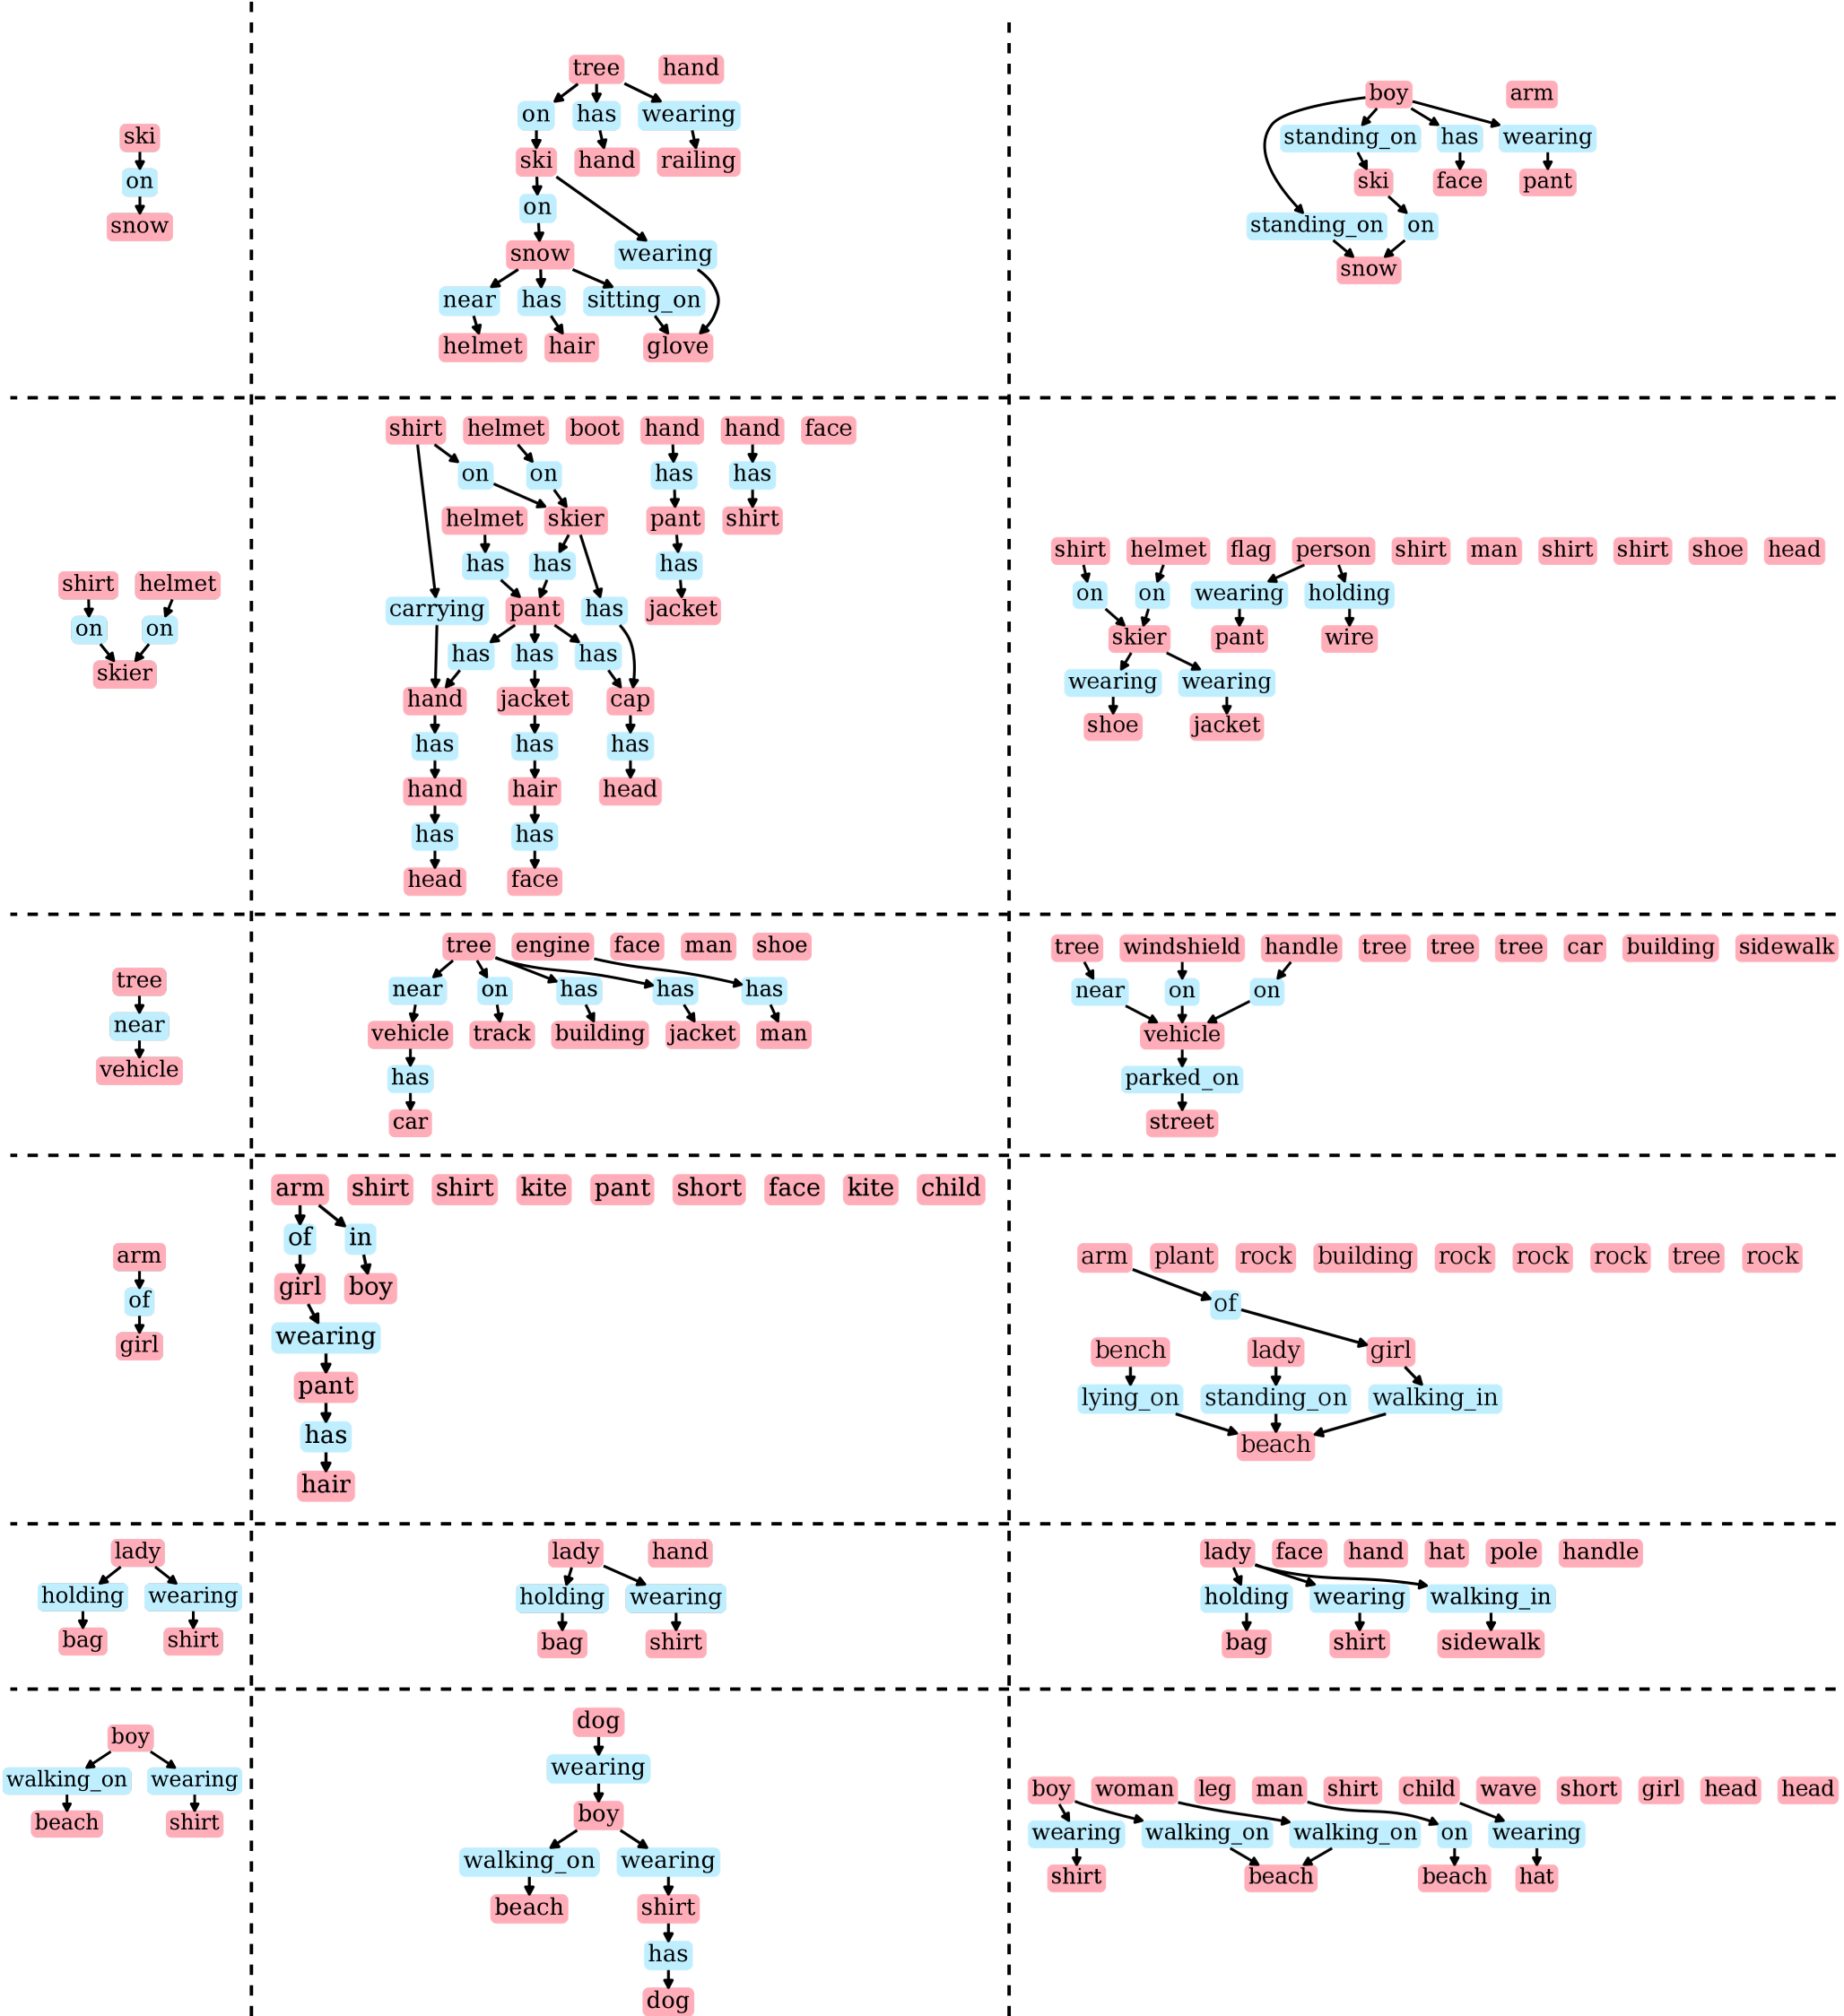

Seed Graph

GraphRNN\*

GEMS
